# Supplementary material for: Micromagnetic structure of oxidized magnetite nanoparticles: sharp structural versus diffuse magnetic interface
Source: arXiv:2506.20571 source file (2025-06-25)
Supplement: Supplementary file 1 [file Supplementary_Information_to___Micromagnetic_structure_of_oxidized_magnetite_nanoparticles__sharp_structural_versus_diffuse_magnetic_interface__.pdf]

# Supplementary Information to “Micromagnetic structure of oxidized magnetite nanoparticles: sharp structural versus diffuse magnetic interface”

Elizabeth M. Jefremovas,<sup>1,2,\*</sup> Michael P. Adams,<sup>1</sup> Lucía Gandarias,<sup>3</sup> Lourdes Marcano,<sup>4</sup> Javier Alonso,<sup>5</sup> Andreas Michels,<sup>1</sup> and Jonathan Leliaert<sup>6</sup>

<sup>1</sup>Department of Physics and Materials Science, University of Luxembourg,  
162A Avenue de la Faiencerie, L-1511 Luxembourg, Grand Duchy of Luxembourg

<sup>2</sup>Institute for Advanced Studies, University of Luxembourg,  
Campus Belval, L-4365 Esch-sur-Alzette, Luxembourg

<sup>3</sup>Aix-Marseille Université, CEA, CNRS, BIAM, 13115 Saint Paul lez Durance, France

<sup>4</sup>Center for Cooperative Research in Biomaterials (CIC biomaGUNE),  
Basque Research and Technology Alliance, Donostia-San Sebastián 20014, Spain

<sup>5</sup>Department CITIMAC, Faculty of Sciences, University of Cantabria, 39005 Santander, Spain

<sup>6</sup>DyNaMat, Department of Solid State Sciences, Ghent University, 9000 Ghent, Belgium

In this Supplementary Information we display additional results of the structural (TEM, XRD) and magnetic characterization of the magnetic nanoparticle samples as well as the expressions for the spin-flip SANS cross section and pair-distance distribution function.

## I. STRUCTURAL CHARACTERIZATION

### A. Morphology of the bacterial magnetosomes

Transmission electron microscopy (TEM) was performed using a JEOL JEM-14000Plus electron microscope at an accelerating voltage of 120 kV. For TEM imaging, the magnetotactic bacteria were dispersed (before freeze-drying) onto 300 micron meshed carbon-coated copper grids. The particle-size distribution was analyzed using the standard software ImageJ [1] for digital electron microscope image processing.

Figure 1(A) displays a representative TEM image of a MSR-1 bacteria. The particle size distribution shown in panel (B) has been obtained from the analysis of 478 intracellular magnetosomes in about 50 bacteria; it is bimodal with one maximum centered at  $16 \pm 4$  nm and a second one at  $42 \pm 8$  nm. This bimodal distribution results from the fact that the magnetosomes at the end of the chains are smaller compared to the ones in the center (see Fig. 1(A)) [2]. The average number of magnetosomes per chain is between 12–20, and there is only one chain along the bacterial body.

Figure 1(C) shows a representative TEM image of a AMB-1 bacteria. From the analysis of the histogram presented in Fig. 1(D), a monomodal size distribution centered at  $42 \pm 6$  nm is obtained from the analysis of 272 intracellular magnetosomes in about 40 bacteria, in agreement with the larger magnetosomes of MSR-1. In both bacterium, the morphology of the magnetosome is similar to a truncated octahedral cube with well-defined facets [3–6] and surrounded by a proteolipidic membrane of  $\cong 4$  nm thickness [3], which acts as a barrier against oxidation [7]. Besides the size distribution, there is a major difference in both strains connected to the chain.

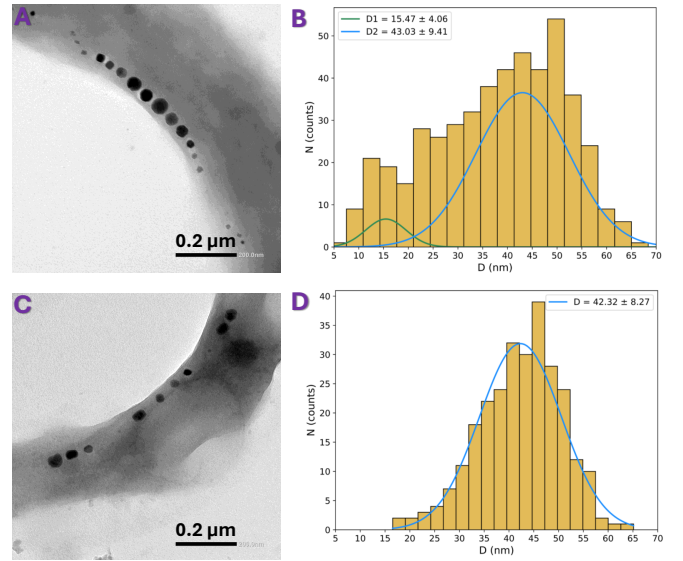

FIG. 1. Representative transmission electron microscopy images of *Magnetospirillum gryphiswaldense* (MSR-1) (A) and *Magnetospirillum magneticum* (AMB-1) (C) together with their corresponding (particle size) histograms in (B) and (D).

Whereas MSR-1 grows one chain of 12–20 magnetosomes per bacteria, AMB-1 grows typically three shorter chains of 3–5 magnetosomes. The origin of this different behavior is attributed to a biomineralization process [8–11] and results in a bimodal size distribution for MSR-1 and in a monomodal one for AMB-1.

### B. X-ray diffraction at room temperature

The crystalline structure of the  $\text{Fe}_3\text{O}_4$  phase has been verified for both bacteria by means of x-ray diffraction (XRD). The measurements were performed at room temperature and under ambient atmosphere. Figure 2

\* elizabeth.jefremovas@uni.lu

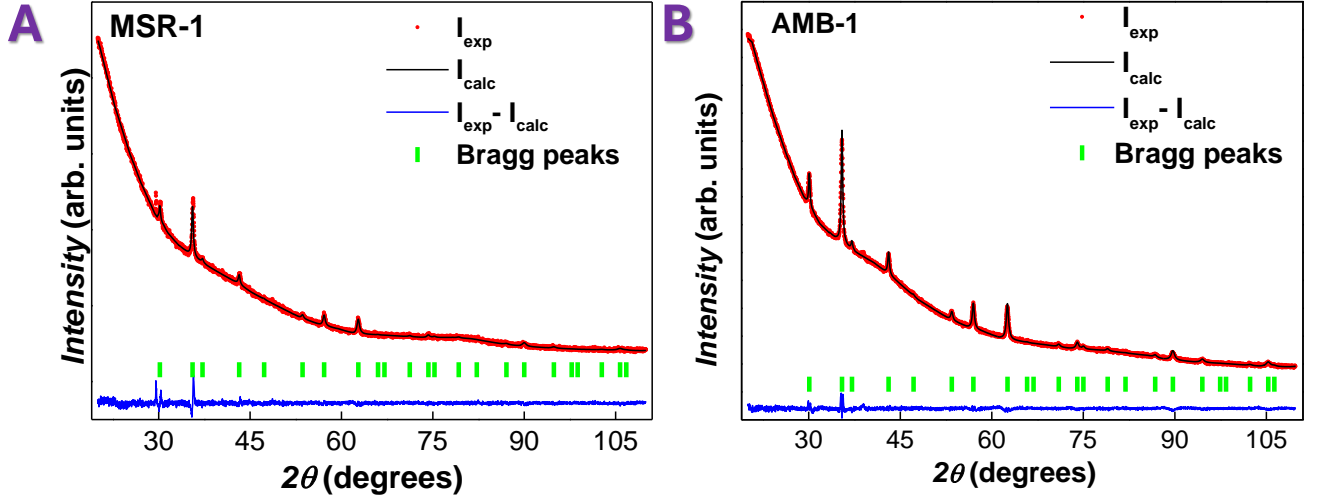

FIG. 2. X-ray diffraction data for (A) *MSB-1* and (B) *AMB-1*. In red, the experimental data together with the calculated Rietveld refinements in black for a single-phase  $Fd-3m$  space group. The blue line represents the difference between the experimental data and the calculated refinement. Marked in green, the corresponding (hkl) peaks for the  $Fd-3m$  space group.

includes the measurements performed for MSR-1 and AMB-1. In both cases, Rietveld refinements are consistent with a single phase of the cubic  $Fd-3m$  space group, with lattice parameters compatible with the magnetite phase [12, 13]:  $a = 8.3985(2)$  Å (Bragg factor  $R_B = 4.5\%$ ) and  $a = 8.3746(1)$  Å ( $R_B = 7.7\%$ ) for MSR-1 and AMB-1, respectively. The presence of maghemite is discarded in both samples, as no peaks that correspond to such a phase are observed, and the obtained lattice parameters are well above the one of maghemite ( $a = 8.3451(3)$  Å) [14]. The magnetic characterization (see Fig. 3 below) plus previous x-ray absorption analysis on bacteria samples of the same strains [5, 15] further validate the absence of maghemite and the purity of the magnetite phase of the fresh magnetosomes ( $t = 0$ ) inside the bacteria. Our Rietveld refinements provide additional information on the mean particle size  $\langle D \rangle$  and on the inhomogeneous microstrain  $\eta$ . The calculated values are  $\langle D \rangle = 45.1(3)$  nm (MSR-1) and  $\langle D \rangle = 49.8(3)$  nm (AMB-1) with respective microstrain parameters of  $\eta = 0.38(1)\%$  and  $\eta = 0.41(1)\%$ . These values are slightly above yet in agreement with the ones obtained by TEM, ensuring the single-crystal domain of the studied magnetotactic bacteria.

## II. HYSTERESIS LOOPS AT ROOM TEMPERATURE

Figure 3 shows the hysteresis loops of MSR-1 measured at  $T = 300$  K after  $t = 0$  years and after  $t = 6$  years, il-

lustrating the most extreme scenario of oxidation from all the cases reported in this work. As it can be observed in Fig. 3(A), the saturation magnetization after 6 years reduces to 0.95 of its initial value, indicating a very minor (if any) reduction of the saturation magnetization. Figure 3(B) shows that both hysteresis curves overlap with a coercivity of  $\mu_0 H_c \cong 17$  mT. The cubic anisotropy term  $K_c$  dominates the macroscopic behavior of the magnetosomes, remaining the coercivity unaffected by the presence of the oxide layer.

## III. SPIN-FLIP SANS CROSS SECTION AND PAIR-DISTANCE DISTRIBUTION FUNCTION

For the particular scattering geometry where the applied magnetic (guide) field  $\vec{H} \parallel \vec{e}_z$  is perpendicular to the incident neutron beam ( $\vec{k}_0 \parallel \vec{e}_x$ ), the elastic differential spin-flip SANS cross section  $d\Sigma_{sf}/d\Omega$  in a uniaxial polarization-analysis experiment can be expressed as follows (compare to Fig. 3 in the main paper) [16]:

$$\frac{d\Sigma_{sf}}{d\Omega} = \frac{8\pi^3}{V} b_H^2 \left( |\tilde{M}_x|^2 + |\tilde{M}_y|^2 \cos^4 \theta + |\tilde{M}_z|^2 \sin^2 \theta \cos^2 \theta - (\tilde{M}_y \tilde{M}_z^* + \tilde{M}_y^* \tilde{M}_z) \sin \theta \cos^3 \theta \right), \quad (1)$$

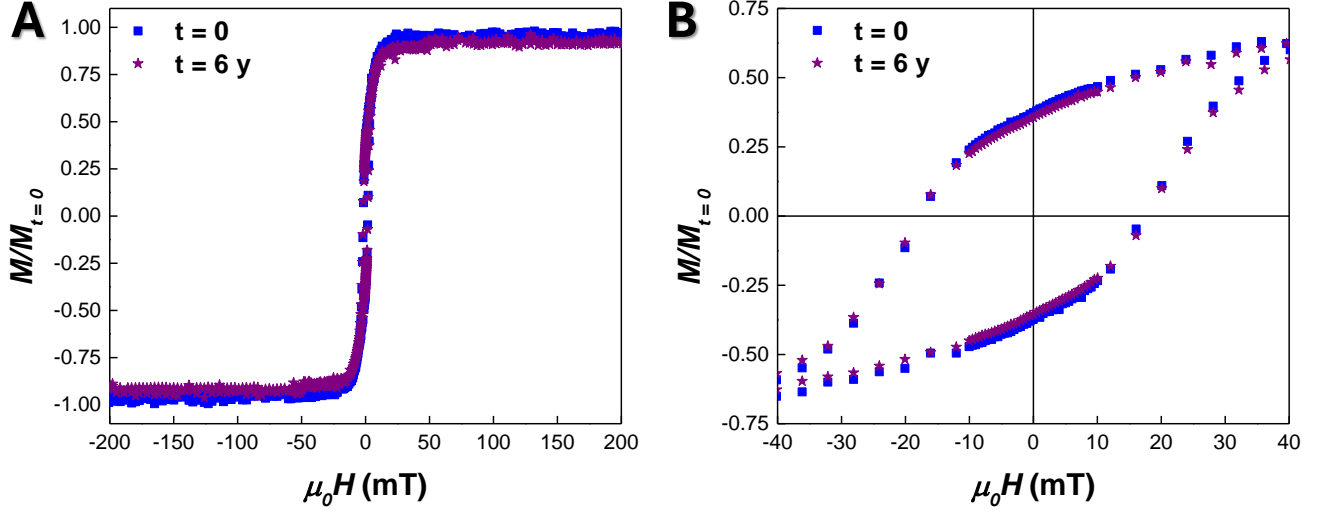

FIG. 3. Hysteresis loops of MSR-1 at  $t = 0$  years and at the maximum oxidation stage of  $t = 6$  years (see inset). In (A) the full loop can be inspected, whereas in (B) the central region is zoomed-in to compare the coercivity in both cases.

where  $V$  is the scattering volume,  $b_H = 2.91 \times 10^8 \text{ A}^{-1}\text{m}^{-1}$  is the magnetic scattering length in the small-angle regime (the atomic magnetic form factor is approximated by 1, since we are dealing with forward scattering),  $\vec{M}(\vec{q}) = \{\vec{M}_x, \vec{M}_y, \vec{M}_z\}$  denotes the Fourier transform of the magnetization vector field  $\vec{M}(\vec{r}) = \{M_x, M_y, M_z\}$ ,  $\theta$  is the angle between  $\vec{H} = H\vec{e}_z$  and  $\vec{q}$ , so that  $\vec{q} \cong q\{0, \sin\theta, \cos\theta\}$  in small-angle approximation, and the asterisks “\*” mark the complex-conjugated quantity. The polarization-dependent chiral function has been neglected in Eq. (1). The Fourier components  $\vec{M}_{x,y,z}(\vec{q})$  are numerically computed from the results  $M_{x,y,z}(\vec{r})$  of the micromagnetic (real-space) simulations.

In small-angle approximation,  $d\Sigma_{\text{sf}}/d\Omega$  is a function of only two independent scattering vector components (see above), say,  $q_y$  and  $q_z$  or, equivalently,  $q$  and  $\theta$ . The quantity  $\frac{d\Sigma_{\text{sf}}}{d\Omega}(q, \theta)$  can then be azimuthally averaged according to:

$$I_{\text{sf}}(q) = \frac{1}{2\pi} \int_0^{2\pi} \frac{d\Sigma_{\text{sf}}}{d\Omega}(q, \theta) d\theta, \quad (2)$$

where  $\theta$  is the azimuthal angle in the detector plane (see Fig. 3 in the main paper). The one-dimensional spin-flip SANS cross section  $I_{\text{sf}}(q)$  can be further analyzed by using the inverse Fourier transform to compute the pair-distance distribution function. This quantity pro-

vides insights into the structure of the real space and the characteristic distances within the sample [17]. The pair-distance distribution function  $p(r)$  is obtained from numerically solving the following equation:

$$p(r) = r^2 \int_0^\infty I_{\text{sf}}(q) j_0(qr) q^2 dq, \quad (3)$$

where  $j_0(x) = \sin(x)/x$  denotes the zero-order spherical Bessel function.

For the case of a uniformly magnetized cuboid, the magnetization profile in reciprocal space governing the spin-flip SANS cross section reads [18]:

$$\vec{M}(\vec{q}) = \frac{V_c}{(2\pi)^{3/2}} \vec{M}_0 j_0\left(\frac{q_x a_x}{2}\right) j_0\left(\frac{q_y a_y}{2}\right) j_0\left(\frac{q_z a_z}{2}\right), \quad (4)$$

where  $V_c = a_x a_y a_z$  denotes the volume of the cuboid, with the  $a_i$  being the dimensions of the cuboid ( $i \in x, y, z$ ), and  $\vec{M}_0$  is a constant vector specifying the saturation direction. Note that for the here considered scattering geometry (Fig. 3 in the main paper with  $q_x = 0$ ), the first spherical Bessel function in Eq. (4) reduces to unity.

With the aforementioned considerations, the  $p(r)$  of the cuboid is obtained as follows:

$$p(r; \vec{M}_0 = M_0 \vec{e}_z) = \frac{V_c b_H^2 M_0^2}{2\pi} r^2 \int_0^\infty \int_0^{2\pi} \left[ j_0 \left( \frac{q a_y \sin \theta}{2} \right) j_0 \left( \frac{q a_z \cos \theta}{2} \right) \right]^2 \sin^2 \theta \cos^2 \theta d\theta j_0(qr) q^2 dq, \quad (5)$$

$$p(r; \vec{M}_0 = M_0 \vec{e}_y) = \frac{V_c b_H^2 M_0^2}{2\pi} r^2 \int_0^\infty \int_0^{2\pi} \left[ j_0 \left( \frac{q a_y \sin \theta}{2} \right) j_0 \left( \frac{q a_z \cos \theta}{2} \right) \right]^2 \cos^4 \theta d\theta j_0(qr) q^2 dq, \quad (6)$$

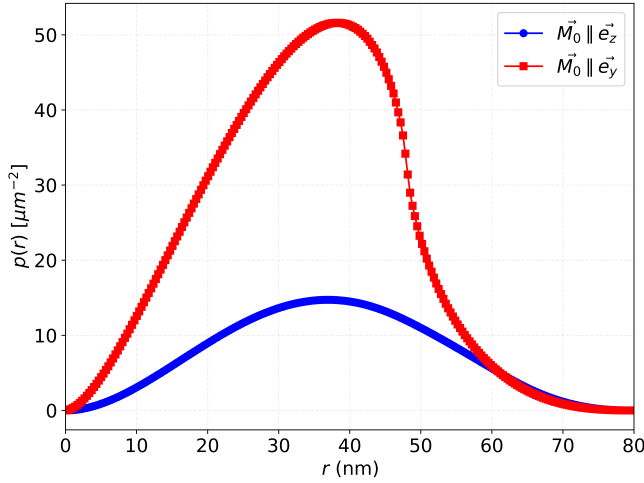

FIG. 4. Pair-distance distribution functions  $p(r)$  of a uniformly-magnetized cuboid of dimensions  $a_x = a_z = 48$  nm and  $a_y = 64$  nm computed from Eqs. (5) and (6). We consider the cases of saturation ( $\vec{M}_0$ ) along  $\vec{e}_z$  (a short axis) and along  $\vec{e}_y$  (long axis). The saturation value of the particle is taken as  $M_0 = 486$  kA/m.

where  $\vec{M}_0 = M_0 \vec{e}_z$  describes the situation where the magnetization is uniform along the field direction (a short axis of the cuboid), and  $\vec{M}_0 = M_0 \vec{e}_y$  is the case where the cuboid is magnetized along the long  $\vec{e}_y$  axis.

Figure 4 shows the  $p(r)$  of a uniformly-magnetized cuboid for the two cases that the saturation direction  $\vec{M}_0$  is along  $\vec{e}_z$  (a short axis) and along  $\vec{e}_y$  (long axis). When the magnetization is pointing along the  $\vec{e}_z$  direction, the corresponding  $p(r)$  is bell-shaped and here centered at around  $r_{\max} \cong 37$  nm. When the magnetization points along the  $\vec{e}_y$  direction (long axis),  $p(r)$  increases in magnitude and its maximum shifts to slightly larger  $r$  values ( $r_{\max} \cong 39$  nm).

- 
- [1] C. A. Schneider, W. S. Rasband, and K. W. Eliceiri, *Nature Methods* **9**, 671 (2012).
  - [2] P. Bender, L. Marcano, I. Orue, D. A. Venero, D. Honecker, L. F. Barquín, A. Muela, and M. L. Fdez-Gubieda, *Nanoscale Advances* **2**, 1115 (2020).
  - [3] I. Orue, L. Marcano, P. Bender, A. García-Prieto, S. Valencia, M. Mawass, D. Gil-Cardón, D. A. Venero, D. Honecker, A. García-Arribas, *et al.*, *Nanoscale* **10**, 7407 (2018).
  - [4] L. Marcano, I. Orue, D. Gandia, L. Gandarias, M. Weigand, R. M. Abrudan, A. García-Prieto, A. García-Arribas, A. Muela, M. L. Fdez-Gubieda, and S. Valencia, *ACS Nano* **16**, 7398 (2022).
  - [5] D. Gandia, L. Marcano, L. Gandarias, D. Villanueva, I. Orue, R. M. Abrudan, S. Valencia, I. Rodrigo, J. Angel García, A. Muela, M. L. Fdez-Gubieda, and J. Alonso, *ACS Applied Materials & Interfaces* **15**, 566 (2022).
  - [6] D. Gandia, L. Gandarias, L. Marcano, I. Orue, D. Gil-Cardón, J. Alonso, A. García-Arribas, A. Muela, and M. L. Fdez-Gubieda, *Nanoscale* **12**, 16081 (2020).
  - [7] J. Cypriano, M. Bahri, K. Dembele, W. Baaziz, P. Leão, D. A. Bazylinski, F. Abreu, O. Ersen, M. Farina, and J. Werckmann, *Scientific Reports* **10**, 6706 (2020).
  - [8] A. Scheffel, M. Gruska, D. Faivre, A. Linaroudis, J. M. Plitzko, and D. Schüler, *Nature* **440**, 110 (2006).
  - [9] D. Faivre, L. H. Böttger, B. F. Matzanke, and D. Schüler, *Angewandte Chemie International Edition* **46**, 8495 (2007).
  - [10] J. Li, Y. Pan, G. Chen, Q. Liu, L. Tian, and W. Lin, *Geophysical Journal International* **177**, 33 (2009).
  - [11] A. Komeili, *Annual Review Biochemistry* **76**, 351 (2007).
  - [12] J. Yoshida and S. Iida, *Journal of the Physical Society of Japan* **47**, 1627 (1979).
  - [13] F. Walz, *Journal of Physics: Condensed Matter* **14**, R285 (2002).
  - [14] C. Goss, *Physics and Chemistry of Minerals* **16**, 164 (1988).
  - [15] M. L. Fdez-Gubieda, A. Muela, J. Alonso, A. García-Prieto, L. Olivi, R. Fernandez-Pacheco, and J. M. Barandiarán, *ACS Nano* **7**, 3297 (2013).
  - [16] A. Michels, *Magnetic Small-Angle Neutron Scattering: A Probe for Mesoscale Magnetism Analysis* (Oxford University Press, Oxford, 2021).
  - [17] D. I. Svergun and M. H. J. Koch, *Reports on Progress in Physics* **66**, 1735 (2003).
  - [18] W. Gille, *Journal of Applied Crystallography* **32**, 1100 (1999).
